# Supplementary material for: Consistent Maximum Likelihood Estimation Using Subsets with Applications to Multivariate Mixed Models
Source: arXiv:1810.01203 ancillary file (2019-02-11)
Supplement: Supplementary file 1 [file suppl_subset_mglmm.pdf]

# SUPPLEMENT TO "CONSISTENT MAXIMUM LIKELIHOOD ESTIMATION USING SUBSETS WITH APPLICATIONS TO MULTIVARIATE MIXED MODELS"

BY KARL OSKAR EKVALL AND GALIN L. JONES

*University of Minnesota*

This note contains additional results and more detailed proofs of some results in "Consistent Maximum Likelihood Estimation Using Subsets with Applications to Multivariate Mixed Models". Throughout, we refer to that article as Ekvall and Jones (2019).

**1. Theory.** Results in this section pertain primarily to Section 2 in Ekvall and Jones (2019).

1.1. *Preliminary results.* We present some lemmas that are used when proving the main results.

LEMMA 1. *For any positive random variables  $X, Y, Z$ , defined on the same probability space, and  $c > 0$ ,  $P(XY \geq Z) \leq P(X \geq c) + P(Y \geq Z/c)$ .*

PROOF. If for positive constants  $x, y, z, c$  it holds that  $xy \geq z$ , then either  $x \geq c$  or  $y \geq z/c$ , since otherwise  $xy < c(z/c) = z$ . Thus,  $\{\omega : X(\omega)Y(\omega) \geq Z(\omega)\} \subseteq \{\omega : X(\omega) \geq c\} \cup \{\omega : Y(\omega) \geq Z(\omega)/c\}$ . By sub-additivity of measures,  $P(XY \geq Z) \leq P(\{X \geq c\} \cup \{Y \geq Z/c\}) \leq P(X \geq c) + P(Y \geq Z/c)$ .  $\square$

LEMMA 2. *Suppose  $A_i, i = 1, \dots, n$  are compact subsets of some metric space  $(\mathcal{T}, d_{\mathcal{T}})$  such that  $\cap_{i=1}^n A_i = \emptyset$ , then the open covers  $C_i = \cup_{x \in A_i} B_{\delta}(x)$ ,  $i = 1, \dots, n$ , also have an empty intersection for all small enough  $\delta > 0$ .*

PROOF. Consider the covers  $C_{k,i} = \cup_{x \in A_i} B_{1/k}(x)$ ,  $k = 1, 2, \dots, i = 1, \dots, n$ . If  $C_k = \cap_i C_{k,i} = \emptyset$  for some  $k < \infty$ , then we are done. Suppose for contradiction  $C_k$  is non-empty for every  $k < \infty$ . By construction, every point  $x_k \in C_k$  is within  $1/k$  of at least one point in every  $A_i$ . That is, we can pick, for every  $k \geq 1$  and  $i = 1, \dots, n$ , an  $x_k \in C_k$  and  $y_{k,i} \in A_i$  such that  $d(x_k, y_{k,i}) \leq 1/k$ . Thus, by the triangle inequality, for every  $k$ ,  $d(y_{k,i}, y_{k,j}) \leq 2/k$ . By compactness of  $A_1$ , say,  $y_{k,1}$  has a convergent subsequence  $y_{k_m,1} \rightarrow y_1$  as  $m \rightarrow \infty$ , for some  $y_1 \in A_1$  by the fact that  $A_1$  is closed as a compact subset of a metric space. But then, for every  $i$ , by the triangle inequality,  $d(y_{k_m,i}, y_1) \leq d(y_{k_m,i}, y_{k_m,1}) + d(y_{k_m,1}, y_1) \leq 2/k_m + d(y_{k_m,1}, y_1) \rightarrow 0$  as  $m \rightarrow \infty$ . Thus, since every  $A_i$  is closed,  $y_1 \in A_i$  for every  $i$ , which is the desired contradiction.  $\square$

LEMMA 3. *Suppose  $\Theta$  is a compact subset of some metric space and, for every  $\theta \in \Theta$ ,  $f_{\theta}$  is a probability density against some dominating measure  $\nu$  which does not*

depend on  $\theta$ . Suppose also that  $f_\theta(x)$  is continuous in  $\theta$  for every  $x$  and define the measures  $\nu_\theta$  by  $\nu_\theta(A) = \int_A f_\theta(x) d\nu(x)$  for any  $\nu$ -measurable  $A$ . Then for any  $\theta^0 \in \Theta$ , the set  $\Theta^0 = \{\theta \in \Theta : \nu_\theta = \nu_{\theta^0}\}$  is compact.

PROOF. Because  $\Theta$  is a compact subset of a metric space, it suffices to show that  $\Theta^0$  is closed. Note that  $\Theta^0$  always includes the point  $\theta^0$  and is thus non-empty. Pick an arbitrary converging sequence  $\theta_n \in \Theta^0$ , call the limit point  $\theta^*$ . By continuity of  $\theta \mapsto f_\theta(x)$  for every  $x$ ,  $f_{\theta_n} \rightarrow f_{\theta^*}$  pointwise. Now for any  $\nu$ -measurable  $A$ ,  $|\nu_{\theta^*}(A) - \nu_{\theta^0}(A)| \leq |\nu_{\theta^*}(A) - \nu_{\theta_n}(A)| + |\nu_{\theta^0}(A) - \nu_{\theta_n}(A)| = |\nu_{\theta^*}(A) - \nu_{\theta_n}(A)|$ , which vanishes as  $n \rightarrow \infty$  by a generalized dominated convergence theorem [6, Theorem 19] – the dominating sequence of functions for which the integrals converge can be  $f_{\theta_n}(x) \geq f_{\theta_n}(x)I_A(x)$  – so indeed  $\theta^* \in \Theta^0$ .  $\square$

1.2. *Main results.* For economical notation in the proofs we write  $f_\theta(y) = f_\theta^n(y)$ ,  $f_\theta(y_i) = f_{\theta,i}(y_i)$ ,  $f_\theta(w) = g_\theta(w)$ ,  $f_\theta(u) = \phi_\theta^r(u)$ , and so on. That is, the letter  $f$  is overloaded and the argument indicates which density we are referring to.

PROOF LEMMA 2.1 IN EKVALL AND JONES (2019). Let  $Y = (W, Z)$ , where  $Z$  consists of the components of  $Y$  that are not in the subcollection  $W$ . Then  $f_\theta(y) = f_\theta(w, z)$  and by (conditional) Markov's inequality, for any  $k > 0$ ,

$$\mathbf{P}(L_n(\theta; Y) \geq c \mid W) \leq c^{-1} \mathbf{E}(L_n(\theta; Y) \mid W) = c^{-1} \mathbf{E}\left(\frac{f_\theta(W, Z)}{f_{\theta^0}(W, Z)} \mid W\right).$$

Now the following calculation shows the random variable

$$L_m(\theta; W) = f_\theta(W) / f_{\theta^0}(W)$$

is a version of  $\mathbf{E}(f_\theta(W, Z) / f_{\theta^0}(W, Z) \mid W)$ :

$$\begin{aligned} \int_{\mathcal{Z}} \frac{f_\theta(w, z)}{f_{\theta^0}(w, z)} f_{\theta^0}(z \mid w) \nu_Z(dz) &= \int_{\mathcal{Z}} \frac{f_\theta(w, z)}{f_{\theta^0}(w, z)} \frac{f_{\theta^0}(w, z)}{f_{\theta^0}(w)} \nu_Z(dz) \\ &= \int_{\mathcal{Z}} \frac{f_\theta(w, z)}{f_{\theta^0}(w)} \nu_Z(dz) \\ &= \frac{f_\theta(w)}{f_{\theta^0}(w)}, \end{aligned}$$

where  $\nu_Z$  is the measure against which the components in  $Z$  have joint density  $f_\theta(z)$  and  $\mathcal{Z}$  is the range space of  $Z$ . Since the conditional expectation is unique up to  $\mathbf{P}$ -null sets, this finishes the proof.  $\square$

PROOF OF LEMMA 2.2 IN EKVALL AND JONES (2019). Fix some arbitrary  $\varepsilon > 0$ . If  $\sup_{\theta \in A_i} L_n(\theta; Y) < 1$  for  $i = 1, \dots, s$ , then, since  $L_n(\theta^0; Y) = 1$ , there are no global maximizers in  $\cup_{i=1}^s A_i \supseteq \Theta \cap B_\varepsilon(\theta^0)^c$ . Thus, it suffices to prove

$$\mathbf{P}\left(\bigcup_{i=1}^s \left\{\sup_{\theta \in A_i} L_n(\theta; Y) \geq 1\right\}\right) \leq \sum_{i=1}^s \mathbf{P}\left(\sup_{\theta \in A_i} L_n(\theta; Y) \geq 1\right) \rightarrow 0.$$

Since  $s$  is fixed it is enough that  $\mathbf{P}(\sup_{\theta \in A_i} L_n(\theta; Y) \geq 1) \rightarrow 0$  for every  $i = 1, \dots, s$ . Without loss of generality, consider  $i = 1$ . Pick a cover of  $A_1$  as given by Assumption 3 and, for every ball in the cover, pick a  $\theta^j$  in the intersection of that ball with  $A_1$ . If there are some balls that do not intersect  $A_1$ , they may be discarded from the cover, so we assume without loss of generality that all balls do intersect  $A_1$ . We then get  $M_{n,1}$  points such that every point in  $A_1$  is within  $\delta_{n,1}$  of at least one of them. For any  $\theta \in A_1$ , let  $\theta^j(\theta)$  denote the  $\theta^j$  closest to it (pick an arbitrary one if there are many). Using the Lipschitz continuity given by Assumption 2 and that  $x \mapsto e^x$  is increasing we have,

$$\begin{aligned} \mathbf{P}\left(\sup_{\theta \in A_1} L_n(\theta; Y) \geq 1\right) &= \mathbf{P}\left(\sup_{\theta \in A_1} \Lambda_n(\theta; Y) \geq 0\right) \\ &= \mathbf{P}\left(\sup_{\theta \in A_1} \ell_n(\theta; Y) \geq \ell_n(\theta^0; Y)\right), \end{aligned}$$

which is upper bounded by

$$\leq \mathbf{P}\left(\sup_{\theta \in A_1} [\ell_n(\theta^j(\theta); Y) + K_{n,1} d_{\mathcal{T}}(\theta, \theta^j(\theta))] \geq \ell_n(\theta^0; Y)\right).$$

Because there are only  $M_{n,1}$  points  $\theta^j$ , and  $d_{\mathcal{T}}(\theta^j(\theta), \theta) \leq \delta_{n,1}$  since  $\theta^j(\theta)$  is the one closest to  $\theta$ , we get that the last line is upper bounded by

$$\begin{aligned} &\mathbf{P}\left(\max_{j \leq M_{n,1}} [\ell_n(\theta^j; Y) + K_{n,1} \delta_{n,1}] \geq \ell_n(\theta^0; Y)\right) \\ &= \mathbf{P}\left(\max_{j \leq M_{n,1}} f_{\theta^j}(Y) e^{K_{n,1} \delta_{n,1}} \geq f_{\theta^0}(Y)\right). \end{aligned}$$

But by applying Lemma 1 with  $c = 2$ ,

$$\begin{aligned} &\mathbf{P}\left(\max_{j \leq M_{n,1}} f_{\theta^j}(Y) e^{K_{n,1} \delta_{n,1}} \geq f_{\theta^0}(Y)\right) \\ &\leq \mathbf{P}\left(2 \max_{j \leq M_{n,1}} f_{\theta^j}(Y) \geq f_{\theta^0}(Y)\right) + \mathbf{P}\left(e^{K_{n,1} \delta_{n,1}} \geq 2\right) \\ &= \mathbf{P}\left(2 \max_{j \leq M_{n,1}} f_{\theta^j}(Y) \geq f_{\theta^0}(Y)\right) + o(1) \end{aligned}$$

where the last line uses Assumption 3. The choice of the constant 2 in the application of Lemma 1 is arbitrary – any number with positive logarithm works. The remaining term,

$$\mathbf{P}\left(2 \max_{j \leq M_{n,1}} f_{\theta^j}(Y) \geq f_{\theta^0}(Y)\right) = \mathbf{P}\left(\max_{j \leq M_{n,1}} L_n(\theta^j; Y) \geq 1/2\right),$$

we will deal with using Lemma 2.1 and dominated convergence. After conditioning on  $W^{(1)}$  we have

$$\begin{aligned} \mathbb{P} \left( \max_{j \leq M_{n,1}} L_n(\theta^j; Y) \geq 1/2 \mid W^{(1)} \right) &\leq \sum_{i=1}^{M_{n,1}} 2L_{m_1}(\theta^j; W^{(1)}) \\ &\leq 2M_{n,1} \sup_{\theta \in A_1} L_{m_1}(\theta, W^{(1)}), \end{aligned}$$

$\mathbb{P}$ -almost surely, where the first inequality is by subadditivity and Lemma 2.1, and the second uses that  $L_n(\theta^j; W^{(1)}) \leq \sup_{\theta \in A_1} L_{m_1}(\theta; W^{(1)})$  by definition. The expression in the last line vanishes as  $n \rightarrow \infty$  by Assumption 3. Thus,

$$\mathbb{P} \left( \max_{j \leq M_{n,1}} L_n(\theta^j; Y) \geq 1/2 \right) \rightarrow 0$$

by dominated convergence. The dominating function can be the constant 1. This finishes the proof.  $\square$

**2. Applications.** Results in this section pertain primarily to Section 3 in Ekvall and Jones (2019). Let  $\lambda_{\max}(\cdot)$  and  $\lambda_{\min}(\cdot)$  denote the maximum and minimum eigenvalue of its matrix argument, respectively. For matrices,  $\|\cdot\|$  denotes the spectral norm and  $\|\cdot\|_F$  the Frobenius norm. Differentiation with respect to  $\theta_i$  is denoted  $\nabla_i$ .

We will use the following well known fact repeatedly. It is stated as a lemma for easy reference.

**LEMMA 4.** *If  $h$  is a continuous function from some metric space  $\mathcal{X}$  to  $\mathbb{R}$  and  $A$  is a compact subset of  $\mathcal{X}$ , then  $\sup_{x \in A} h(x) = h(x^*)$  for some  $x^* \in A$ . In particular, if  $h(x) < c$  for some constant  $c$  and every  $x \in A$ , then  $\sup_{x \in A} h(x) < c$ .*

Of course, the same holds if the supremum is replaced by an infimum or if less than is replaced by greater than.

**LEMMA 5.** *Let  $X_{n,1}, \dots, X_{n,n}$  be a triangular array with rows of i.i.d. multivariate normal  $q$ -vectors with mean  $\mathbb{E}(X_{n,i}) = \mu = \mu(\theta)$  and covariance matrix  $\text{cov}(X_{n,i}) = \Sigma = \Sigma(\theta)$ ,  $\theta \in \Theta$ . Suppose that*

$$0 < 1/c_1 \leq \inf_{\theta \in \Theta} \lambda_{\min}(\Sigma(\theta)) \leq \sup_{\theta \in \Theta} \lambda_{\max}(\Sigma(\theta)) \leq c_1 < \infty$$

and  $\sup_{\theta \in \Theta} \|\mu(\theta)\| \leq c_2$  for some  $c_1, c_2 \in (0, \infty)$ , then

$$\sup_{\theta \in \Theta} \left| n^{-1} \sum_{i=1}^n \{ \Lambda_i(\theta; X_{n,i}) - \mathbb{E}[\Lambda_1(\theta; X_{n,1})] \} \right| \rightarrow 0,$$

$\mathbb{P}$ -almost surely, where  $\Lambda_i(\theta; X_{n,i}) = \log f_\theta(X_{n,i})/f_{\theta^0}(X_{n,i})$ , and  $f_\theta(X_{n,i})$  means the density for  $X_{n,i}$  evaluated at  $X_{n,i}$ .

PROOF. Theorem 16 in Ferguson [2] applies almost verbatim to triangular arrays in place of i.i.d. sequences. The only necessary modification to its proof is that the pointwise strong law of large numbers needs to be motivated. Write

$$\begin{aligned}
 \sup_{\theta \in \Theta} |\Lambda_1(\theta; x)| &\leq \sup_{\theta \in \Theta} |\log f_\theta(x)| + |\log f_{\theta^0}(x)| \\
 &\leq \sup_{\theta \in \Theta} |\log \det \Sigma| + \sup_{\theta \in \Theta} \|x - \mu\|^2 \|\Sigma^{-1}\| + |\log f_{\theta^0}(x)| \\
 &\leq \sup_{\theta \in \Theta} |\log \det \Sigma| + \sup_{\theta \in \Theta} (\|x\| + \|\mu\|)^2 \sup_{\theta \in \Theta} \|\Sigma^{-1}\| + |\log f_{\theta^0}(x)| \\
 &\leq |\log(qc_1)| + (\|x\| + c_2)^2 c_1 + |\log f_{\theta^0}(x)| \\
 &=: K(x),
 \end{aligned}$$

which is a quadratic function of  $x$ , not depending on  $\theta$ . Thus, since the  $X_{n,i}$ s are i.i.d. and normal random variables have all finite moments,  $\Lambda_i(\theta; X_{n,i})$  has bounded fourth moment, uniformly in  $i$ ,  $n$ , and  $\theta$ . Classical proofs for a strong law with finite fourth moment applies without change to triangular arrays. The other conditions of Ferguson's Theorem 16 are easy to verify, using  $K(x)$  as the dominating function.  $\square$

PROOF PROPOSITION 3.1 IN EKVALL AND JONES (2019). Lemma 3 gives that  $\{\theta \in \Theta : \nu_\theta^i = \nu_{\theta^0}^i\}$  is a closed set,  $i = 1, \dots, s$ . Thus, the sets  $D_i = \{\theta \in \Theta : \nu_\theta^i = \nu_{\theta^0}^i\} \cap B_\varepsilon(\theta^0)^c$ ,  $i = 1, \dots, s$ , are closed as intersections of closed sets and compact as a closed subsets of a compact set,  $\Theta$ . By Lemma 2 we can pick  $\delta$  small enough that the open covers  $B_i = \cup_{\theta \in D_i} B_\delta(\theta) \supseteq D_i$  have an empty intersection,  $\cap_{i=1}^s B_i = \emptyset$ . Let  $A_i = \Theta \cap B_\varepsilon(\theta^0)^c \cap B_i^c$  and note  $\cup_{i=1}^s A_i = \Theta \cap B_\varepsilon(\theta^0)^c \cap (\cup_{i=1}^s B_i^c) = \Theta \cap B_\varepsilon(\theta^0)^c \cap (\cap_{i=1}^s B_i)^c = \Theta \cap B_\varepsilon(\theta^0)^c$ . Each  $A_i$  closed as the intersection of closed sets, and compact as a closed subset of a compact set,  $\Theta$ . By construction, for any  $\theta \in A_i$  it must be that  $\theta \in B_i^c \subseteq D_i^c$ . Since  $A_i$  is a subset of  $B_\varepsilon(\theta^0)^c$  by construction this implies  $\theta \in \{\theta \in \Theta : \nu_\theta^i = \nu_{\theta^0}^i\}^c$ , which finishes the proof.  $\square$

### 2.1. Longitudinal linear mixed model.

LEMMA 6. *The log-likelihood  $\ell_n(\theta; y)$  is differentiable in  $\theta$  at any interior point of  $\Theta$ , for every  $n \geq 1$  and every  $y$  in the support of  $Y$ .*

PROOF. The multivariate normal log-likelihood  $\ell_n(\theta; Y)$  is differentiable in its mean  $m$  and covariance matrix  $C$  everywhere  $C = C(\theta)$  is positive definite [4]. It is easy to see that  $C$  is positive definite on all interior point since  $\Psi$  is (c.f. Lemma 7). Now  $\ell_n(\theta; Y)$  is differentiable on all interior points by the chain rule since the elements of  $m$  and  $C$  are differentiable in  $\theta$ .  $\square$

PROOF LEMMA 3.2 IN EKVALL AND JONES (2019). Fix an  $\varepsilon > 0$  small enough that all points of  $\bar{B}_\varepsilon(\theta^0)$  are interior. By construction of the subcollections, the assumptions of Proposition 3.1 are satisfied with what is there denoted  $\Theta$  replaced by  $\bar{B}_\varepsilon(\theta^0)$ . Take  $A_1$  and  $A_2$  to be the compact sets given by that proposition. The

proof of point 1 is standard [2, p. 115] and hence omitted. Point 2 is proven by checking the conditions of Lemma 5 with what is there denoted  $\Theta$  replaced by the compact  $A_i, i = 1, 2$ . The following argument works for either subcollection. First note  $\lambda_{\max}(C_i) = \|C_i(\theta)\| \leq \|C_i(\theta)\|_F$  [1]. Since the Frobenius norm is the square root of the sum of squared entries and the entries are continuous functions of  $\theta$ ,  $\theta \mapsto \|C_i(\theta)\|_F$  is continuous and attains its supremum on the compact set  $A_i$ , so  $\|C(\theta)\|$  is bounded above on  $\bar{B}_\varepsilon(\theta^0)$ . By spectral decomposition of  $C_i$  it is immediate that  $\lambda_{\min}(C_i) = 1/\lambda_{\max}(C_i^{-1})$ . Thus, since  $C_i(\theta)$  is clearly positive definite on all interior points and the inverse is a continuous mapping at points where  $C_i$  is positive definite [4], we get by the same arguments that  $\lambda_{\max}(C_i^{-1}(\theta))$  is bounded on  $A_i$ . It is obvious that  $\theta \mapsto m_i(\theta)$  is continuous and hence attains its supremum on  $A_i$ . This concludes the proof of point 2.

It remains to prove point 3. By point 1 we may pick an  $\epsilon > 0$  such that, for either subcollection,

$$\sup_{\theta \in A_i} N^{-1} \mathbb{E}[\Lambda_{N/2}(\theta; W^{(i)})] = \sup_{\theta \in A_i} \mathbb{E}[\Lambda_1(\theta; W_1^{(i)})]/2 < -3\epsilon.$$

By point 2 we have, P-almost surely and for all large enough  $N$ ,

$$\sup_{\theta \in A_i} N^{-1} |\Lambda_{N/2}(\theta; W^{(i)}) - \mathbb{E}[\Lambda_{N/2}(\theta; W^{(i)})]| \leq \epsilon.$$

Thus we have that  $\sup_{\theta \in A_i} \Lambda_{N/2}(\theta; W^{(i)}) < -2N\epsilon$ , and hence that

$$\sup_{\theta \in A_i} L_{N/2}(\theta; X^{(i)}) \leq e^{-2N\epsilon},$$

for all large enough  $N$ , P-almost surely. The last right hand side is clearly  $o(e^{-\epsilon N})$  as  $N \rightarrow \infty$ .  $\square$

We will use the following results in the proof of Lemma 3.3 in Ekvall and Jones (2019).

LEMMA 7. *The following hold when all points in  $\bar{B}_\varepsilon(\theta^0)$  are interior (the first inequality in 1 holds always):*

1.  $\|\Psi\|_F \leq T$  and  $\sup_{\theta \in \bar{B}_\varepsilon(\theta^0)} \|\Psi^{-1}\|_F \leq c\sqrt{T}$  for some  $c > 0$ ,
2.  $\sup_{\theta \in \bar{B}_\varepsilon(\theta^0)} \|C(\theta)\| \leq c_1 NT + c_2 T + c_3$  for some  $c_1, c_2, c_3 > 0$ ,
3.  $\sup_{\theta \in \bar{B}_\varepsilon(\theta^0)} \|C(\theta)^{-1}\| \leq c$  for some  $c > 0$ ,
4.  $\sup_{\theta \in \bar{B}_\varepsilon(\theta^0)} \|\nabla_i \Sigma\| \leq NT + cT^2$  for some  $c > 0$  and every  $i \geq 3$ .
5.  $\sup_{\theta \in \bar{B}_\varepsilon(\theta^0)} \|Y - m(\theta)\| = o_{\mathbb{P}}(n)$ , and

PROOF. 1. The Frobenius norm is the square root of the sum of squared elements, and all elements of  $\Psi$  are in the form  $\theta_7^k$  for some integer  $k$  – this establishes the first inequality. The inverse of  $\Psi$  can be written as  $(1 - \theta_7^2)^{-1}$

times a tri-diagonal matrix where the diagonal entries are 1 or  $1 + \theta_7^2$ , and the leading off-diagonals have entries  $-\theta_7$ . Thus,  $\|\Psi^{-1}\|_F$  is the square root of the sum of  $3T$  possibly non-zero elements, each a continuous function of  $\theta$ . The inequality now follows from Lemma 4.

2. Using that eigenvalues of the sum of two positive, semi-definite matrices must be at least as large as those of either summand and that the eigenvalues of Kronecker products are the products of the multiplicands' eigenvalues [4], we get

$$\begin{aligned}\lambda_{\max}(C) &\leq \lambda_{\max}(\theta_3 I_n) + \lambda_{\max}(\theta_4 I_N \otimes J_{NT}) + \lambda_{\max}(\theta_5 J_N \otimes I_N \otimes J_T) \\ &\quad + \lambda_{\max}(\theta_6 I_{N^2} \otimes \Psi) \\ &\leq \theta_3 + \theta_4 NT + \theta_5 NT + \theta_6 T,\end{aligned}$$

where in the last step we also used  $\lambda_{\max}(\Psi) \leq \|\Psi\|_F \leq T$  by 1. The existence of the constants  $c_1, c_2, c_3$  now follows from Lemma 4.

3. Since  $Z\Sigma Z^\top$  is positive definite, we get  $\lambda_{\min}(C) = \lambda_{\min}(\theta_3 I_n + Z\Sigma Z^\top) \geq \theta_3$ . Since all points in  $\bar{B}_\varepsilon(\theta^0)$  are interior,  $\theta_3$  is lower bounded by some  $c^{-1} > 0$  on it (Lemma 4). Thus, using that the eigenvalues of  $C^{-1}$  are the reciprocals of the eigenvalues of  $C$ , we get  $\|C^{-1}\|_F \leq (nc^2)^{1/2} = N\sqrt{T}c$ .
4. Clearly,  $\nabla_3 C(\theta) = I_n$  which has eigenvalue 1 with multiplicity  $n$ . If  $i = 4$  or  $i = 5$ , then the derivative is either  $I_N \otimes J_N \otimes J_T$  or  $J_N \otimes I_N \otimes J_T$ , which both have maximal eigenvalue  $NT$ . If  $i = 6$ , then the derivative is  $\Psi \otimes I_{N^2}$ , which has maximal eigenvalue less than  $T$  by 1. If  $i = 7$ , then the derivative is  $\theta_6 \nabla_7 \Psi$ . We have  $\nabla_7 \Psi_{i,j} = |i-j|\theta_7^{|i-j|-1}$  if  $|i-j| \geq 1$  and  $\nabla_7 \Psi_{i,j} = 0$  otherwise. Thus,  $\nabla_7 \Psi_{i,j} \leq T$  and, consequently,  $\|\nabla_7 \Psi\|_F \leq T^2$ . We conclude, by Lemma 4,  $\nabla_7 C(\theta) \leq cT^2$  for some  $c > 0$ .
5. Let  $U\Lambda U^\top$  be the spectral decomposition of  $C$ . Then  $\|Y - m(\theta)\| = \|U^\top(Y - m(\theta))\|$ . The vector  $U^\top(Y - m(\theta))$  is multivariate normal with mean 0 and covariance matrix  $\Lambda$ . Thus, since a Gaussian process is determined by its finite dimensional distributions, the stochastic process  $\|Y - m(\theta)\|^2$ ,  $\theta \in \bar{B}_\varepsilon(\theta^0)$ , has the same distribution as the process  $\sum_{i=1}^n \Lambda_{i,i}(\theta) \xi_i^2$ , where  $\xi_1, \dots, \xi_n$  are i.i.d. standard normal. By point 2, the supremum of the latter process satisfies  $\sup_{\theta \in \bar{B}_\varepsilon(\theta^0)} \sum_{i=1}^n \Lambda_{i,i}(\theta) \xi_i^2 \leq (c_1 NT + c_2 T + c_3) \sum_{i=1}^n \xi_i^2 = o_P(n^2)$ , which follows from that the last sum is a positive random variable with mean  $n$ , and hence it converges to zero in  $L_1$  when divided by anything of higher order than  $n$ .  $\square$

PROOF PROPOSITION 3.3 IN EKVALL AND JONES (2019). Define  $e = e(\theta) = Y - m(\theta)$  and let  $\nabla_e$  and  $\nabla_C$  denote differentiation with respect to  $e$  and  $C$ . Since  $e$  is linear in  $\theta_1$  and  $\theta_2$ , and  $C(\theta)$  is differentiable in each  $\theta_i$ ,  $i \geq 3$ , bounding the gradient for  $\theta$  is easily done after establishing bounds for  $\nabla_C \ell_n(\theta; Y)$  and  $\nabla_e \ell_n(\theta)$ . These derivatives exist for every  $n$  because the covariance matrix  $C(\theta)$  is positive-definite on  $\bar{B}_\varepsilon(\theta^0)$  by Lemma 7 and the multivariate normal log-likelihood

is differentiable wherever the covariance matrix is non-singular [4]. We have

$$\nabla_C \ell_n(\theta; Y) = -\frac{1}{2} \left[ C^{-1} + C^{-1} e e^\top C^{-1} \right] \text{ and } \nabla_e \ell_n(\theta) = -C^{-1} e.$$

Thus,

$$\begin{aligned} |\nabla_1 \ell_n(\theta)| &= |\nabla_e \ell_n(\theta)^\top \nabla_1 e(\theta)| = |e^\top C^{-1} \mathbf{1}_n| \leq \|e\| \|C^{-1}\| N^2 T, \\ |\nabla_2 \ell_n(\theta)| &= |\nabla_e \ell_n(\theta)^\top \nabla_2 e(\theta)| = |e^\top C^{-1} h_n| \leq \|e\| \|C^{-1}\| N^2 T/2, \end{aligned}$$

and, for  $i \geq 3$ ,

$$\begin{aligned} |\nabla_i \ell_n(\theta)| &= |\text{vec}[\nabla_C \ell_n(\theta)]^\top \text{vec}[\nabla_i C]| = \frac{1}{2} \text{vec} \left[ C^{-1} + C^{-1} e e^\top C^{-1} \right]^\top \text{vec}[\nabla_i C] \\ &= \text{tr} \left[ (C^{-1} + C^{-1} e e^\top C^{-1}) \nabla_i C \right] \\ &\leq \|C^{-1}\|_F \|\nabla_i C\|_F + |e^\top C^{-1} \nabla_i C^{-1} e| \\ &\leq \|C^{-1}\|_F \|\nabla_i C\|_F + \|e\|^2 \|C^{-1}\|^2 \|\nabla_i C\|, \end{aligned}$$

where  $\text{vec}(\cdot)$  denotes the vectorization operator stacking the columns of its matrix argument. Thus, by Lemma 7,

$$\begin{aligned} \sup_{\theta \in \bar{B}_\varepsilon(\theta)} |\nabla_1 \ell_n(\theta)| &\leq \sup_{\theta \in \bar{B}_\varepsilon(\theta)} \|e\| \|C^{-1}\| N^2 T \leq o_P(n) O(NT + T) T N^2 = o_P(T^3 N^5), \\ \sup_{\theta \in \bar{B}_\varepsilon(\theta)} |\nabla_2 \ell_n(\theta)| &\leq \sup_{\theta \in \bar{B}_\varepsilon(\theta)} \|e\| \|C^{-1}\| N^2 T/2 \leq o_P(n) O(NT + T) T N^2 = o_P(T^3 N^5), \end{aligned}$$

and, for  $i \geq 3$ ,

$$\sup_{\theta \in \bar{B}_\varepsilon(\theta)} |\nabla_i \ell_n(\theta)| \leq \sup_{\theta \in \bar{B}_\varepsilon(\theta)} (\|C^{-1}\|_F \|\nabla_i C\|_F + \|e\|^2 \|C^{-1}\|^2 \|\nabla_i C\|).$$

By Lemma 7 the supremum of each of the terms in the last line are of at most polynomial order, which finishes the proof.  $\square$

## 2.2. Logit-Normal MGLMM.

LEMMA 8. *The log-likelihood  $\ell_n(\theta; y)$  is differentiable in  $\theta$  on  $\bar{B}_\varepsilon(\theta^0)$ , for every  $n \geq 1$  and every  $y$  in the support of  $Y$ .*

PROOF. To prove differentiability of  $f_\theta(y)$  in  $\theta$  on  $\bar{B}_\varepsilon(\theta^0)$ , checking the usual conditions for differentiation under the integral are sufficient [3, Theorem 2.27]. It's obvious that  $f_\theta(y | u) f_\theta(u)$  is differentiable in  $\theta$  on every interior point of  $\Theta$ , so it suffices to find, for  $i = 1, \dots, d$ , functions  $K_i : \mathbb{R}^{2n} \times \mathbb{R}^{2N} \rightarrow [0, \infty)$ , not depending on  $\theta$ , such that  $|\nabla_i f_\theta(y | u) f_\theta(u)| \leq K_i(y, u)$  and  $\int K_i(y, u) du < \infty$ . Clearly,  $|\nabla_i f_\theta(y | u) f_\theta(u)| \leq \|\nabla_{\beta_1} f_\theta(y | u) f_\theta(u)\|$ , for any  $i$  such that  $\theta_i$  is a component of  $\beta_1$ , and similarly for the components of  $\beta_2$ . Thus, it suffices to find bounds for  $\|\nabla_{\beta_i} f_\theta(y | u) f_\theta(u)\|$ ,  $i = 1, 2$ , and  $|\nabla_{\theta_d} f_\theta(y | u) f_\theta(u)|$ . For the purposes of this integration, the responses  $y_{i,j,k}$  are constant and the sample size  $n$  is fixed. We prove the existence of integrable bounds in the following forms, where  $c_1, \dots, c_4 > 0$ ,

1.  $K_1(y, u) = c_1 \exp\left(-\frac{1}{2c_2} u^\top u\right) \sum_{i,j} \left(|y_{i,j,1}| + 1 + |u_i^{(1)}| + |u_j^{(2)}|\right) \geq \|\nabla_{\beta_1} f_\theta(y | u) f_\theta(u)\|,$
2.  $K_2(y, u) = c_3 \exp\left(-\frac{1}{2c_2} u^\top u\right) \geq \|\nabla_{\beta_2} f_\theta(y | u) f_\theta(u)\|,$  and
3.  $K_3(y, u) = c_4 \exp\left(-\frac{1}{2c_2} u^\top u\right) (u^\top u + 1) \geq |\nabla_{\theta_d} f_\theta(y | u) f_\theta(u)|.$

It is clear that  $K_1, K_2, K_3$  so defined are integrable because they are, up to scaling, moments of multivariate normal distributions. Thus, it remains only to prove the stated inequalities indeed hold.

By the triangle inequality, that  $f_\theta(y | u) \leq (2\pi)^{-n/2}$ , and the fact that  $f_\theta(u)$  does not depend on  $\beta_1$ , we have

$$\begin{aligned} \|\nabla_{\beta_1} f_\theta(y | u) f_\theta(u)\| &= \left\| f_\theta(y | u) f_\theta(u) \sum_{i,j} (y_{i,j,1} - \eta_{i,j,1}) x_{i,j} \right\| \\ &\leq (2\pi)^{-n/2} (2\pi\theta_d)^{-N} \exp\left(-\frac{1}{2\theta_d} u^\top u\right) \\ &\quad \times \sum_{i,j} (|y_{i,j,1}| + \|\beta_1\| \|x_{i,j}\| + |u_i^{(1)}| + |u_j^{(2)}|) \|x_{i,j}\| \end{aligned}$$

The inequality in the definition of  $K_1$  follows from Lemma 4 upon noting that  $\theta_d$  is bounded both away from zero and above on interior points, that  $\|\beta_1\|$  is similarly upper bounded on such points, and that  $\|x_{i,j}\| \leq 1$  by assumption.

For the inequality in the definition of  $K_2$  we use that  $f_\theta(y | u) \leq (2\pi)^{-n/2}$  and that  $|y_{i,j,2} - 1/(1 + e^{-\eta_{i,j,2}})| \leq 1$ . The latter assertion follows from that  $y_{i,j,2} \in \{0, 1\}$  and that  $1/(1 + e^t) \in (0, 1)$  for all  $t \in \mathbb{R}$ . Thus, since  $f_\theta(u)$  does not depend on  $\beta_2$ ,

$$\begin{aligned} \|\nabla_{\beta_2} f_\theta(y | u) f_\theta(u)\| &= \left\| f_\theta(y | u) f_\theta(u) \sum_{i,j} (y_{i,j,2} - 1/(1 + e^{-\eta_{i,j,2}})) x_{i,j} \right\| \\ &\leq n(2\pi)^{-n/2} (2\pi\theta_d)^{-N} \exp\left(-\frac{1}{2\theta_d} u^\top u\right) \|x_{i,j}\|. \end{aligned}$$

Now the desired inequality follows from again noting the bounds from below and above of  $\theta_d$  and that  $\|x_{i,j}\| \leq 1$ .

The inequality in the definition of  $K_3$  follows similarly. First,  $f_\theta(y | u)$  does not depend on  $\theta_d$  so we get

$$\begin{aligned} |\nabla_{\theta_d} f_\theta(y | u) f_\theta(u)| &= \left| f_\theta(y | u) f_\theta(u) \left(-\frac{N}{\theta_d} + \frac{u^\top u}{2\theta_d^2}\right) \right| \\ &\leq (2\pi)^{-n/2} (2\pi\theta_d)^{-N} \exp\left(-\frac{u^\top u}{2\theta_d}\right) \left(\frac{N}{\theta_d} + \frac{u^\top u}{2\theta_d^2}\right). \end{aligned}$$

Now we are done upon again appealing to the lower and upper bounds of  $\theta_d$  on  $\bar{B}_\varepsilon(\theta^0)$ .  $\square$

We will need the following lemmas.

LEMMA 9. *Let  $\mathcal{X}$  be a metric space and  $f : \mathcal{X} \times \mathbb{R}^d \rightarrow \mathbb{R}$ , for some  $d > 0$ , be continuous under the product metric. If  $\mathcal{X}$  is compact, then  $h(y) = \sup_{x \in \mathcal{X}} f(x, y)$  is continuous.*

PROOF. Fix some  $y$  and consider the compact set  $A = \mathcal{X} \times \bar{B}_1(y)$ . Since  $A$  is compact,  $f$  is uniformly continuous on  $A$ . Thus, for any  $\epsilon > 0$  we can pick  $\delta$  such that for every  $(x', y'), (x'', y'') \in A$ , it holds that if  $d((x', y'), (x'', y'')) < \delta$ , then  $|f(x', y') - f(x'', y'')| < \epsilon$ . Thus, for any  $y' \in B_\delta(y) \subseteq B_1(y)$ , we have  $|h(y) - h(y')| = |\sup_{x \in \mathcal{X}} f(x, y) - \sup_{x \in \mathcal{X}} f(x, y')| \leq \sup_{x \in \mathcal{X}} |f(x, y) - f(x, y')| = |f(x^*(y, y'), y) - f(x^*(y, y'), y')| < \epsilon$ , where  $x^*(y, y') = \arg \max_{x \in \mathcal{X}} |f(x, y) - f(x, y')|$ . The  $\arg \max$  exists by Lemma 4 since continuity of  $f$  implies continuity in  $x$  for every  $y$ .  $\square$

LEMMA 10. *The K–L divergence from a Bernoulli distribution with parameter  $p$  to one with parameter  $q$  is lower bounded by  $2(p - q)^2$ .*

PROOF. By direct computation, the K–L divergence is  $p \log(p/q) + (1 - p) \log([1 - p]/[1 - q])$ . Now using that  $t(1 - t) \leq 1/4$  for all  $t \in \mathbb{R}$  and assuming  $p > q$  we get

$$\begin{aligned} p \log(p/q) + (1 - p) \log([1 - p]/[1 - q]) &= \int_q^p \left( \frac{p}{t} - \frac{1 - p}{1 - t} \right) dt \\ &= \int_q^p \left( \frac{p - t}{t(1 - t)} \right) dt \\ &\geq 4 \int_q^p (p - t) dt \\ &= 2(p - q)^2 \end{aligned}$$

If instead  $q > p$ , then the same inequality results from letting  $1 - p$  and  $1 - q$  take the roles of  $p$  and  $q$ . If  $p = q$ , then the inequality is an equality.  $\square$

Let  $C(\delta, G, \|\cdot\|)$  denote the  $\delta$ -covering number of the set  $G$  under the distance associated with the norm  $\|\cdot\|$ , that is, the least number of open balls of radius  $\delta$  needed to cover  $G$ .

LEMMA 11 (Theorem 8.2 [5]). *Let  $h_1(\omega, \theta), h_2(\omega, \theta), \dots, \theta \in A \subseteq \Theta$ , be independent processes with integrable envelopes  $H_1(\omega), H_2(\omega), \dots$ , meaning  $|h_i(\omega, \theta)| \leq H_i(\omega)$ , for all  $i$  and  $\theta \in A$ . Let  $H = (H_1, \dots, H_N)$  and*

$$\mathcal{H}_{N, \omega} = \{[h_1(\omega, \theta), \dots, h_N(\omega, \theta)] \in \mathbb{R}^N : \theta \in A\}.$$

*If for every  $\epsilon > 0$  there exists a  $K > 0$  such that*

1.  $N^{-1} \sum_{i=1}^N \mathbb{E}[H_i I(H_i > K)] < \epsilon$  for all  $N$ , and

2.  $\log C(\epsilon \|H\|_1, \mathcal{H}_{N,\omega}, \|\cdot\|_1) = o_P(N)$  as  $N \rightarrow \infty$ ,

then

$$\sup_{\theta \in A} N^{-1} \left| \sum_{i=1}^N h_i(\omega, \theta) - \mathbb{E}(h_i(\omega, \theta)) \right| \xrightarrow{P} 0.$$

PROOF. Pollard [5] proves this result with packing numbers replaced by covering numbers. Since [5, p. 10]

$$C(\epsilon, \mathcal{H}_{N,\omega}, \|\cdot\|_1) \leq D(\epsilon, \mathcal{H}_{N,\omega}, \|\cdot\|_1) \leq C(\epsilon/2, \mathcal{H}_{N,\omega}, \|\cdot\|_1),$$

where  $D$  denotes packing numbers, there is nothing more to prove.  $\square$

PROOF LEMMA 3.5 IN EKVALL AND JONES (2019). Let us first prove that, given  $\varepsilon > 0$ , there exists a  $\zeta > 0$ , and hence  $A_i = A_i(\varepsilon, \zeta)$ ,  $i = 1, 2$ , such that point 1 in the lemma holds. The definition of  $A_i(\varepsilon, \zeta)$  is as in the main text. Let  $c(t) = \log(1 + e^t)$  denote the cumulant function in the conditional distribution of  $Y_{i,2}$  given the random effects and define

$$p_i(\beta_2, \theta_d) = \mathbb{E} \left[ c' \left( x_{i,i}^\top \beta_2 + \sqrt{\theta_d / \theta_d^0} (U_i^{(1)} + U_j^{(2)}) \right) \right].$$

Recall,  $\mathbb{E}$  denotes expectation with respect to the distributions indexed by  $\theta^0$ , so  $p_i(\beta_2, \theta_d)$  is the success probability of  $Y_{i,2}$  when  $\beta_2$  and  $\theta_d$  are the true parameters.

Note that because the components in  $W^{(2)}$  are independent,  $\mathbb{E}[\Lambda_N(\theta; W^{(2)})]$  is a sum of  $N$  terms, each summand being the negative K–L divergence between two Bernoulli variables with parameters  $p_i(\beta_2, \theta_d)$  and  $p_i(\beta_2^0, \theta_d^0)$ . Thus, by Lemma 10, Jensen's inequality, the reverse triangle inequality, and the triangle inequality, respectively,

$$\begin{aligned} & N^{-1} \mathbb{E}[\Lambda_N(\theta; W^{(2)})] \\ & \leq -2N^{-1} \sum_{i=1}^N [p_i(\beta_2, \theta_d) - p_i(\beta_2^0, \theta_d^0)]^2 \\ & \leq -2 \left[ N^{-1} \sum_{i=1}^N |p_i(\beta_2, \theta_d) - p_i(\beta_2^0, \theta_d^0)| \right]^2 \\ & \leq -2 \left[ N^{-1} \sum_{i=1}^N \left| |p_i(\beta_2, \theta_d) - p_i(\beta_2, \theta_d^0)| - |p_i(\beta_2^0, \theta_d^0) - p_i(\beta_2, \theta_d^0)| \right| \right]^2 \\ (1) \quad & \leq -2 \left[ N^{-1} \sum_{i=1}^N |p_i(\beta_2, \theta_d) - p_i(\beta_2, \theta_d^0)| - N^{-1} \sum_{i=1}^N |p_i(\beta_2^0, \theta_d^0) - p_i(\beta_2, \theta_d^0)| \right]^2. \end{aligned}$$

Let us work separately with the averages in the last line. We will show that the second can be made arbitrarily small on  $A_2$  by selecting  $\zeta$  small enough, and that the first is

bounded away from zero on the same  $A_2$ , leading to an asymptotic upper bound on  $\sup_{\theta \in A_2} N^{-1} \mathbb{E}[\Lambda_N(\theta; W^{(2)})]$  away from zero. We start with the first average.

Let  $H$  be a compact subset of  $\mathbb{R}$  such that  $x_{i,i}^\top \beta_2 \in H$  for all  $i$  and  $\theta \in \bar{B}_\varepsilon(\theta^0)$ . Such  $H$  exists because the predictors are bounded and  $\beta_2$  is bounded on  $\bar{B}_\varepsilon(\theta^0)$ . Then, defining  $\tilde{p}_i(\gamma, \theta_d)$  as  $p_i(\beta_2, \theta_d)$  but with  $x_{i,i}^\top \beta_2$  replaced by  $\gamma$ , we get

$$\sup_{\theta \in A_2} |p_i(\beta_2, \theta_d) - p_i(\beta_2, \theta_d^0)| \leq \sup_{\theta \in A_2} \sup_{\gamma \in H} |\tilde{p}_i(\gamma, \theta_d) - \tilde{p}_i(\gamma, \theta_d^0)|.$$

Since the random variable in the expectation defining  $\tilde{p}_i$  is bounded by 1 (it is the mean of a Bernoulli random variable),  $\tilde{p}_i$  is continuous by dominated convergence. Thus, since  $H$  is compact,  $\sup_{\gamma \in H} |\tilde{p}_i(\gamma, \theta_d) - \tilde{p}_i(\gamma, \theta_d^0)|$  is continuous in  $\theta_d$  by Lemma 9. That is, we can make  $\sup_{\gamma \in H} |\tilde{p}_i(\gamma, \theta_d) - \tilde{p}_i(\gamma, \theta_d^0)|$  arbitrarily small on  $A_2 = A_2(\zeta, \varepsilon)$  by picking  $\zeta$  small enough, which is what we wanted to show. We next work with the second average in (1).

By the mean value theorem, for some  $\tilde{\beta}_{2,i}$  between  $\beta_2$  and  $\beta_2^0$ ,

$$|p_i(\beta_2^0, \theta_d^0) - p_i(\beta_2, \theta_d^0)| = |\mathbb{E}(c''(x_{i,i}^\top \tilde{\beta}_{2,i} + U_i^{(2)} + U_j^{(2)})) x_{i,i}^\top (\beta_2 - \beta_2^0)|.$$

Here, differentiation under the expectation is permissible since  $c''$  is the variance of a Bernoulli random variable, hence bounded by 1/4, and  $|x_{i,i}^\top (\beta_2 - \beta_2^0)| \leq \|x_{i,i}\| \|\beta_2 - \beta_2^0\| \leq \varepsilon$  on  $\bar{B}_\varepsilon(\theta^0)$ . By the same bound on  $c''$  we get that  $\mathbb{E}(c''(\gamma + U_i^{(1)} + U_j^{(2)}))$  is continuous in  $\gamma$ . Thus, by Lemma 4,  $\inf_{\gamma \in H} \mathbb{E}(c''(\gamma + U_i^{(1)} + U_j^{(2)})) \geq c_1 > 0$ . That  $c_1$  must be positive follows from that  $c''$  is strictly positive on all of  $\mathbb{R}$ . We have thus proven that  $|p_i(\beta_2^0, \theta_d^0) - p_i(\beta_2, \theta_d^0)| \geq c_1 |x_{i,i}^\top (\beta_2 - \beta_2^0)|$ , uniformly on  $\bar{B}_\varepsilon(\theta^0)$ . Using this and that  $|x_{i,i}^\top (\beta_2 - \beta_2^0)| \leq \|x_{i,i}\| \|\beta_2 - \beta_2^0\| \leq \varepsilon \leq 1$  so that squaring it makes it smaller,

$$\begin{aligned} N^{-1} \sum_{i=1}^N |p_i(\beta_2^0, \theta_d^0) - p_i(\beta_2, \theta_d^0)| &\geq c_1 N^{-1} \sum_{i=1}^N |x_{i,i}^\top (\beta_2 - \beta_2^0)| \\ &\geq c_1 N^{-1} (\beta_2 - \beta_2^0)^\top \left( \sum_{i=1}^N x_{i,i} x_{i,i}^\top \right) (\beta_2 - \beta_2^0) \\ &\geq c_1 \|\beta_2 - \beta_2^0\|^2 N^{-1} \lambda_{\min} \left( \sum_{i=1}^N x_{i,i} x_{i,i}^\top \right) \end{aligned}$$

which lower limit as  $N \rightarrow \infty$  is bounded below by some strictly positive constant, say  $c_2$ , since  $\liminf_{N \rightarrow \infty} N^{-1} \lambda_{\min} \left( \sum_{i=1}^N x_{i,i} x_{i,i}^\top \right) \geq c_3 > 0$ , for some  $c_3$ , and  $\|\beta_2 - \beta_2^0\| \geq \varepsilon/2 > 0$  on  $A_2$ . To summarize, we may pick  $\zeta$  so small that the second average in (1) is less than  $c_2/2$ , say, and hence get  $\sup_{\theta \in A_2} N^{-1} \mathbb{E}[\Lambda_N(\theta; W^{(2)})] \leq -2(c_2 - c_2/2)^2 < 0$ , for all but at most finitely many  $N$ . This proves point 1 as it pertains to  $A_2$ .

Consider next

$$A_1 = \partial B_\varepsilon(\theta^0) \cap (\{\theta : |\theta_d - \theta_d^0| \geq \zeta\} \cup \{\theta : \|\beta_2 - \beta_2^0\| \leq \varepsilon/2\})$$

and  $W^{(1)}$ . Similarly to for  $W^{(2)}$ ,  $\mathbb{E}[\Lambda_N(\theta; W^{(1)})]$  can due to independence be written as a sum of  $N$  terms in the form

$$(2) \quad \begin{aligned} & \mathbb{E}\{\log[f_\theta(Y_{i,i,1})/f_{\theta^0}(Y_{i,i,1})]\} \\ &= -\frac{1}{2} \left[ \log \left( \frac{1+2\theta_d}{1+2\theta_d^0} \right) + \frac{1+2\theta_d^0 + [x_i^\top(\beta_2 - \beta_2^0)]^2}{1+2\theta_d} - 1 \right], \end{aligned}$$

which is the negative K-L divergence between two univariate normal distributions. Let us consider the possible values this can take for  $\theta \in A_1$ . If  $|\theta_d - \theta_d^0| \geq \zeta$ , then (2) is upper bounded by what is obtained when  $\beta_1 = \beta_1^0$ . This in turn is a continuous function in  $\theta_d$  and hence attains its supremum on the compact set  $\{\theta_d : \zeta \leq |\theta_d - \theta_d^0| \leq \varepsilon\}$ , and hence on  $A_1$ . This supremum is strictly positive because the divergence can be zero only if  $\theta_d = \theta_d^0$ . If instead  $\|\beta_2 - \beta_2^0\| \leq \varepsilon/2$ . Then either  $|\theta_d - \theta_d^0| \geq \varepsilon/4$  or  $\|\beta_1 - \beta_1^0\| \geq \varepsilon/4$ , for otherwise it cannot be that  $\|\theta - \theta^0\| = \varepsilon$ . If  $|\theta_d - \theta_d^0| \geq \varepsilon/4$  the divergence in (2) has a lower bound away from zero by the same argument as for the cases  $|\theta_d - \theta_d^0| \geq \zeta$ . It remains to deal with the case  $\|\beta_1 - \beta_1^0\| \geq \varepsilon/4$ .

Write  $[x_{i,i}^\top(\beta_1^0 - \beta_1)]^2 = (\beta_1^0 - \beta_1)^\top x_i x_i^\top (\beta_1^0 - \beta_1)$  to see that

$$-2N^{-1}\Lambda_N(\theta; W^{(1)})$$

is equal to

$$\log \left( \frac{1+2\theta_d}{1+2\theta_d^0} \right) + \frac{1+2\theta_d^0 + N^{-1} \sum_{i=1}^N (\beta_1^0 - \beta_1)^\top x_i x_i^\top (\beta_1^0 - \beta_1)}{1+2\theta_d} - 1,$$

which has a lower limit that is greater than

$$\log \left( \frac{1+2\theta_d}{1+2\theta_d^0} \right) + \frac{1+2\theta_d^0 + c_3(\varepsilon/4)^2}{1+2\theta_d} - 1.$$

This expression is in turn maximized in  $\theta_d$  at  $\theta_d = \theta_d^0 + c_3(\varepsilon/16)^2$ ; this follows from a straightforward optimization in  $1+2\theta_d$ . The corresponding maximum evaluates to  $\log(1+2\theta_d^0 + c_3(\varepsilon/4)^2) - \log(1+2\theta_d^0) > 0$ . This finishes the proof of point 1.

The proof of point 2 consists of checking the conditions of Lemma 11. We first work with  $A_1$  and  $W^{(1)}$ . Let  $h_i(\omega, \theta) = \log[f_\theta(Y_{i,i,1}(\omega))/f_{\theta^0}(Y_{i,i,1}(\omega))]$  be the log-likelihood ratio for the  $i$ th observation in the first subcollection,  $i = 1, \dots, N$ . We equip  $\mathcal{H}_{N,\omega}$  with the  $L_1$  norm  $\|\cdot\|_1$ , and  $\Theta$  is equipped with the  $L_2$  norm as before. To facilitate checking the two conditions we will first derive envelopes with the following properties:  $\sup_{-\infty < i < \infty} \mathbb{E} H_i^k < \infty$  for every  $k \geq 0$ ,  $\sup_{-\infty < i < \infty} \mathbb{P}(H_i \geq K) \rightarrow 0$  as  $K \rightarrow 0$ , and each  $h_i(\omega, \theta)$  is  $H_i$ -Lipschitz in  $\theta$  on  $\bar{B}_\varepsilon(\theta^0)$ , and hence on  $A_1$ , for every  $\omega$ . We start with the Lipschitz property.

Let us use the slight abuse of notation that  $y_{i,i,1} = Y_{i,i,1}(\omega)$ . Since the distribution of  $W^{(1)}$  does not depend on  $\beta_2$  we have  $\nabla_{\beta_2} h_i(\omega, \theta) = 0$ , and for some  $c_1, c_2, c_3, c_4, c_5 > 0$

(depending on  $\varepsilon$ ), and every  $\theta \in \bar{B}_\varepsilon(\theta^0)$ ,

$$\begin{aligned} \|\nabla_{\beta_1} h_i(\omega, \theta)\| &= \|(y_{i,i,1} - x_{i,i}^\top \beta_1) x_{i,i} / (1 + 2\theta_d)\| \leq c_1 |y_{i,i,1}| + c_2 \\ |\nabla_{\theta_d} h_i(\omega, \theta)| &= \frac{1}{2} \left| \frac{1}{1 + 2\theta_d} - (y_{i,i,1} - x_{i,i}^\top \beta_1)^2 / (1 + 2\theta_d)^2 \right| \\ &\leq c_3 + c_4(|y_{i,i,1}| + c_5)^2. \end{aligned}$$

The existence of these constants follow from Lemma 4. Let  $H_i$  be the sum of the bounds, i.e.

$$H_i(\omega) = c_1 |y_{i,i,1}| + c_2 + c_3 + c_4(|y_{i,i,1}| + c_5)^2.$$

By the mean value theorem,  $|h_i(\omega, \theta) - h_i(\omega, \theta')| = |(\theta - \theta')^\top \nabla h_i(\omega, \tilde{\theta})| \leq \|\theta - \theta'\| H_i$  for some  $\tilde{\theta}$  between  $\theta$  and  $\theta'$ . That is,  $h_i$  is  $H_i$ -Lipschitz on  $\bar{B}_\varepsilon(\theta^0)$ . That  $H_i$  is an envelope for  $h_i$  follows from noting that  $h_i(\omega, \theta^0) = 0$  so by taking  $\theta' = \theta^0$  in the previous calculation,  $|h_i(\omega, \theta)| \leq H_i \|\theta - \theta^0\| \leq H_i$  on  $\bar{B}_\varepsilon(\theta^0)$ . That  $\sup_i \mathbb{E}(H_i^k) < \infty$  for every  $k > 0$  and  $\sup_i \mathbb{P}(H_i > K) \rightarrow 0$  as  $K \rightarrow \infty$  follow from that  $Y_{i,i,1}$  is normally distributed with variance  $1 + 2\theta_d^0$ , not depending on  $i$ , and mean satisfying  $-\|\beta_1^0\| \leq x_{i,i}^\top \beta_1^0 \leq \|\beta_1^0\|$ . We are now ready to check the conditions of Lemma 11.

By the Cauchy-Schwartz inequality and the properties just derived, we have for every fixed  $N$  that

$$N^{-1} \sum_{i=1}^N \mathbb{E}[H_i I(H_i > K)] \leq \sup_i \mathbb{E}[H_i^2] \sup_i \mathbb{P}(H_i \geq K) \rightarrow 0, \quad K \rightarrow \infty,$$

which verifies the first condition.

For the second condition, note that the derived Lipschitz property gives, for arbitrary  $h = (h_1(\omega, \theta), \dots, h_N(\omega, \theta))$  and  $h' = (h_1(\omega, \theta'), \dots, h_N(\omega, \theta'))$  in  $\mathcal{H}_{N,\omega}$ :

$$\begin{aligned} \|h - h'\|_1 &= \sum_{i=1}^N |h_i(\omega, \theta) - h_i(\omega, \theta')| \\ &\leq \sum_{i=1}^N \|\theta - \theta'\| H_i(\omega) \\ &= \|\theta - \theta'\| \|H\|_1. \end{aligned}$$

Thus, if we cover  $\partial B_\varepsilon(\theta^0)$  with  $\epsilon$ -balls with centers  $\theta^j$ ,  $j = 1, \dots, M$ , then the corresponding  $L_1$  balls in  $\mathbb{R}^N$  of radius  $\epsilon \|H\|_1$  with centers

$$h^j = (h_1(\omega, \theta^j), \dots, h_N(\omega, \theta^j))$$

cover  $\mathcal{H}_{N,\omega}$ . This is so because for every  $\theta \in \partial B_\varepsilon(\theta^0)$  there is a  $\theta^j$  such that  $\|\theta - \theta^j\| \leq \epsilon$ , and hence by the Lipschitz property  $\|h(\omega, \theta) - h(\omega, \theta^j)\|_1 \leq \|H\|_1 \epsilon$ . Thus,

$C(\epsilon \|H\|_1, \mathcal{H}_{N,\omega}, \|\cdot\|_1) \leq C(\epsilon, \partial B_\epsilon(\theta^0), \|\cdot\|)$ . Since  $C(\epsilon, \partial B_\epsilon(\theta^0), \|\cdot\|)$  is constant in  $N$ , the second condition of Lemma 11 is verified for  $A_1$  and  $W^{(1)}$ .

The arguments for  $A_2$  and  $W^{(2)}$  are similar, redefining  $h_i(\omega, \theta)$  with  $Y_{i,i,1}$  replaced by  $Y_{i,1,2}$ , taking  $A_2$  in place of  $A_1$ , and so on. We need only prove the existence of envelopes  $H_1, \dots, H_N$  with the desired properties. Using that  $|y_{i,j,2} - c'(\eta_{i,2,1})| \leq 1$  and that  $f_\theta(y_{i,i,2} | u)f_\theta(u)/f_\theta(y_{i,i,2}) = f_\theta(u | y_{i,i,2})$  one gets,

$$\begin{aligned} \|\nabla_{\beta_2} h_i(\omega, \theta)\| &= \left\| \nabla_{\beta_2} \log \int f_\theta(y_{i,i,2} | u) f_\theta(u) du \right\| \\ &= \left\| \frac{1}{f_\theta(y_{i,i,2})} \int f_\theta(y_{i,i,2} | u) f_\theta(u) [y_{i,i,2} - c'(\eta_{i,j,2})] x_{i,i} du \right\| \\ &\leq \|x_{i,i}\| \leq 1. \end{aligned}$$

Using that  $U_i^{(1)}$  and  $U_j^{(2)}$  are the only random effects entering the linear predictor  $\eta_{i,j,2}$ , and that  $f_\theta(y_{i,j,2} | u) \leq 1$ ,

$$\begin{aligned} &|\nabla_{\theta_d} h_i(\omega, \theta)| \\ &= \left| \frac{1}{f_\theta(y_{i,i,2})} \int f_\theta(y_{i,i,2} | u) f_\theta(u_i^{(1)}, u_j^{(2)}) \left( \frac{(u_i^{(1)})^2 + (u_j^{(2)})^2}{2\theta_d^2} - \frac{1}{\theta_d} \right) du \right| \\ &\leq \frac{1}{2\theta_d f_\theta(y_{i,i,2})} \int f_\theta(u_i^{(1)}, u_j^{(2)}) \left( \frac{(u_i^{(1)})^2 + (u_j^{(2)})^2}{\theta_d} \right) du + \frac{1}{\theta_d} \\ &= \frac{1}{\theta_d f_\theta(y_{i,j,2})} + \frac{1}{\theta_d}. \end{aligned}$$

By Lemma 4 the quantity in the last line attains its supremum on  $\bar{B}_\epsilon(\theta^0)$ . This maximum is finite for both  $y_{i,i,2} = 1$  and  $y_{i,i,2} = 0$  since the marginal success probability cannot be one or zero on interior points of  $\Theta$ . Thus, on  $\bar{B}_\epsilon(\theta^0)$ ,  $\|\nabla h_i(\omega, \theta)\|$  is bounded by a constant, say  $H$ , the largest needed for the two cases  $y_{i,i,2} = 0$  and  $y_{i,i,2} = 1$ . By setting  $H_i = H, i = 1, \dots, N$ , we have envelopes with the right properties and this completes the proof of point 2.

Finally, we prove point 3. Consider without loss of generality the first subset and subcollection. For economical notation we write  $L_N(\theta) = L_N(\theta; W^{(1)})$  and  $\Lambda_N(\theta) = \Lambda_N(\theta; W^{(1)})$ . Point 1 gives that  $\sup_{\theta \in A_1} \mathbb{E}[\Lambda_N(\theta)] < -3\epsilon$  for some  $\epsilon > 0$  and all large

enough  $N$ . Assuming that  $N$  is large enough that this holds, we get

$$\begin{aligned} \mathbb{P}\left(e^{\epsilon N} \sup_{\theta \in A_1} L_N(\theta) > e^{-\epsilon N}\right) &= \mathbb{P}\left(N^{-1} \sup_{\theta \in A_1} \Lambda_N(\theta) > -2\epsilon\right) \\ &\leq \mathbb{P}\left(N^{-1} \sup_{\theta \in A_1} \Lambda_N(\theta) > \epsilon + \sup_{\theta \in A_1} \mathbb{E}[\Lambda_N(\theta)]\right) \\ &= \mathbb{P}\left(N^{-1} \sup_{\theta \in A_1} \Lambda_N(\theta) - \sup_{\theta \in A_1} \mathbb{E}[\Lambda_N(\theta)] > \epsilon\right) \\ &\leq \mathbb{P}\left(N^{-1} \sup_{\theta \in A_1} |\Lambda_N(\theta) - \mathbb{E}[\Lambda_N(\theta)]| > \epsilon\right), \end{aligned}$$

which vanishes as  $N \rightarrow \infty$  by point 2. Thus, since  $e^{-\epsilon N} \rightarrow 0$ ,

$$e^{\epsilon N} \sup_{\theta \in A_1} L_n(\theta) \xrightarrow{\mathbb{P}} 0.$$

□

PROOF LEMMA 3.6 IN EKVALL AND JONES (2019). We will find a Lipschitz constant (random variable) with the desired properties by bounding  $\|\nabla \log f_\theta(y)\|$ . We first consider derivatives with respect to  $\theta_d$ . Define

$$J^n(\theta) = (2\pi\theta_d)^N f_\theta(y) = \int f_\theta(y | u) \exp\left(-\frac{u^\top u}{2\theta_d}\right) du$$

and

$$K^n(\theta) = \int f_\theta(y | u) \exp\left(-\frac{u^\top u}{2\theta_d}\right) \frac{u^\top u}{2\theta_d^2} du.$$

Then  $\nabla_{\theta_d} J^n(\theta) = K^n(\theta)$ , and hence

$$\nabla_{\theta_d} \log f_\theta(y) = \nabla_{\theta_d} \log[(2\pi\theta_d)^{-N} J^n(\theta)] = -\frac{N}{\theta_d} + \frac{K^n(\theta)}{J^n(\theta)}.$$

We focus on the second term first. Let  $A_n = \{u \in \mathbb{R}^{2N} : u^\top u \leq a_n\}$  for some constant  $a_n$  (depending on the total sample size  $n$ ). Let  $K_1^n(\theta)$  be the integral defining  $K^n(\theta)$  restricted to  $A_n$ , and let  $K_2^n(\theta)$  be the same integral but instead restricted to  $A_n^c$  so that  $K^n(\theta) = K_1^n(\theta) + K_2^n(\theta)$ . Then, since the integrands are non-negative,

$$K_1^n(\theta)/J^n(\theta) = \frac{\int_{A_n} f_\theta(y | u) \exp\left(-\frac{u^\top u}{2\theta_d}\right) \frac{u^\top u}{2\theta_d^2} du}{\int f_\theta(y | u) \exp\left(-\frac{u^\top u}{2\theta_d}\right) du} \leq \frac{a_n}{2\theta_d^2}$$

and, hence,

$$|\nabla_{\theta_d} \log f_\theta(y)| \leq \frac{N}{\theta_d} + \frac{a_n}{2\theta_d^2} + \frac{K_2^n(\theta)}{J^n(\theta)}.$$

On  $A_n^c$  we have by definition that  $u^\top u \geq u^\top u/2 + a_n/2$ . Thus, using that  $f_\theta(y | u) \leq (2\pi)^{-n/2}$ ,

$$\begin{aligned}
 K_2^n(\theta) &\leq \int_{A_n^c} f_\theta(y | u) \exp\left(-\frac{1}{2\theta_d}(u^\top u/2 + a_n/2)\right) \frac{u^\top u}{2\theta_d^2} du \\
 &\leq \frac{1}{2\theta_d^2} e^{-\frac{a_n}{4\theta_d}} \int f_\theta(y | u) \exp\left(-\frac{u^\top u}{4\theta_d}\right) u^\top u du \\
 &\leq \frac{1}{2\theta_d^2} e^{-\frac{a_n}{4\theta_d}} (2\pi)^{-n/2} \int \exp\left(-\frac{u^\top u}{4\theta_d}\right) u^\top u du \\
 &= \frac{1}{2\theta_d^2} e^{-\frac{a_n}{4\theta_d}} (2\pi)^{-n/2} (4\pi\theta_d)^N \int (4\pi\theta_d)^{-N} \exp\left(-\frac{u^\top u}{4\theta_d}\right) u^\top u du \\
 (3) \quad &= \frac{4N\theta_d}{2\theta_d^2} e^{-\frac{a_n}{4\theta_d}} (2\pi)^{-n/2} (4\pi\theta_d)^N.
 \end{aligned}$$

Using Lemma 4, (3) can be upper bounded on  $\bar{B}_\varepsilon(\theta^0)$  by  $h_1^n = \exp(c_1 a_n + c_2 n + c_3 N + c_4 \log N + c_5)$  for some constants  $c_1, \dots, c_5$ . It will be important later to note that the constant  $c_1$  is negative in this expression.

We next derive a lower bound on  $J^n(\theta)$ . To that end, let  $B_n = \{u \in \mathbb{R}^{2N} : |u_i| \leq 1, i = 1, \dots, N\}$ . Since the integrand in  $J^n(\theta)$  is positive, we may lower bound it by the same integral restricted to  $B_n$ . We then get, using that  $\exp(-u^\top u/(2\theta_d)) \geq \exp(-N/\theta_d)$  on  $B_n$  and that Lebesgue measure of  $B_n$  is  $4^N$ ,

$$\begin{aligned}
 J^n(\theta) &\geq \exp\left(-\frac{N}{\theta_d}\right) \int_{B_n} f_\theta(y | u) du \\
 (4) \quad &\geq e^{-\frac{N}{\theta_d}} (2\pi)^{-n/2} \\
 &\quad \times \exp\left(-\sum_{i,j} y_{i,j,1}^2/2 + |y_{i,j,1}|(|x_{i,j}^\top \beta_1| + 2) + (|x_{i,j}^\top \beta_1| + 2)^2\right) \\
 (5) \quad &\quad \times \exp\left(-\sum_{i,j} |y_{i,j,2}|(|x_{i,j}^\top \beta_2| + 2) + \log(1 + e^{|x_{i,j}^\top \beta_2|} + 2)\right) 4^N.
 \end{aligned}$$

Here, the last inequality lower bounds all terms in the exponent by minus their absolute values. Again using Lemma 4, that the predictors are bounded, and that  $|y_{i,j,2}| \leq 1$ , we thus see that  $J^n(\theta)$  can be lower bounded on  $\bar{B}_\varepsilon(\theta^0)$  by  $h_2^n(y) = \exp(c_6 N + c_7 n + c_8 \sum_{i,j} y_{i,j,1}^2 + c_9 \sum_{i,j} |y_{i,j,1}| + c_{10})$ , for some constants  $c_6, \dots, c_{10}$ . Thus, by lower bounding  $\theta_d > c_{11}^{-1}$  on  $\bar{B}_\varepsilon(\theta^0)$  for some  $c_{11} > 0$  we get

$$\sup_{\theta \in \bar{B}_\varepsilon(\theta^0)} |\nabla_{\theta_d} \log f_\theta(y)| \leq c_{11} N + c_{11}^2 a_n/2 + \frac{h_1^n}{h_2^n(y)}.$$

Now, take  $a_n = n^{1+\epsilon/2}$  for some  $\epsilon > 0$ . Then the first two terms are  $O(a_n)$  as  $n \rightarrow \infty$ . Moreover, since  $\sum_{i,j} \mathbf{E} Y_{i,j,1}^2 \leq n(1 + 2\theta_d^0) + n\|\beta_1^0\| = O(n)$  by boundedness of the

predictors, both sums in the exponent of  $h_1^n/h_2^n(y)$  converges to zero in  $L_1$  if divided by  $a_n$ , and hence also in probability. It follows from the continuous mapping theorem that  $h_1/h_2^n(y) = O_P(1)$  since, as remarked above,  $c_1 < 0$ . We have thus proven that  $\sup_{\theta \in \bar{B}_\epsilon(\theta^0)} |\nabla_{\theta_d} \log f_\theta(y)| = O_P(a_n) = o_P(n^{1+\epsilon})$ , for every  $\epsilon > 0$ .

For  $\beta_1$  we get by using the triangle inequality, boundedness of the predictors,  $t(1-t) \leq 1/4$ ,  $t \in \mathbb{R}$ , and  $f_\theta(y | u)f_\theta(u)/f_\theta(y) = f_\theta(u | y)$ ,

$$\begin{aligned}
\|\nabla_{\beta_1} \log f_\theta(y)\| &= \left\| \frac{1}{f_\theta(y)} \int f_\theta(y | u) f_\theta(u) \sum_{i,j} [y_{i,j,1} - \eta_{i,j,1}] x_{i,j} du \right\| \\
&\leq \left| \sum_{i,j} (y_{i,j,1} - x_{i,j}^\top \beta_1) \right| + \left| \frac{1}{f_\theta(y)} \int f_\theta(y | u) f_\theta(u) \sum_{i,j} |u_i^{(1)} + u_j^{(2)}| du \right| \\
&\leq \left| \sum_{i,j} (y_{i,j,1} - x_{i,j}^\top \beta_1) \right| \\
&\quad + \left| \frac{1}{f_\theta(y)} \int f_\theta(y | u) f_\theta(u) \sum_{i,j} [1/2 + (u_i^{(1)})^2 + (u_j^{(2)})^2] du \right| \\
&= \left| \sum_{i,j} (y_{i,j,1} - x_{i,j}^\top \beta_1) \right| + n/2 + \frac{1}{f_\theta(y)} \int f_\theta(y | u) f_\theta(u) u^\top u du \\
&= \left| \sum_{i,j} (y_{i,j,1} - x_{i,j}^\top \beta_1) \right| + n/2 + 2\theta_d^2 \frac{K^n(\theta)}{J^n(\theta)}
\end{aligned}$$

Thus, by Lemma 4 and the same arguments as for  $\nabla_{\theta_d} \log f_\theta(y)$  we get that

$$\sup_{\theta \in B_\epsilon(\theta^0)} \|\nabla_{\beta_1} \log f_\theta(Y)\| = o_P(n^{1+\epsilon})$$

for any  $\epsilon > 0$ .

Finally, by the triangle inequality and that  $|y_{i,j,2} - c'(\eta_{i,j,2})| \leq 1$  for all  $i$  and  $j$ ,

$$\begin{aligned}
\|\nabla_{\beta_2} \log f_\theta(y)\| &= \left\| \frac{1}{f_\theta(y)} \int f_\theta(y | u) \sum_{i,j} [y_{i,j,2} - c'(\eta_{i,j,2})] x_{i,j} f_\theta(u) du \right\| \\
&\leq n
\end{aligned}$$

□

## References.

- [1] R. Bhatia. *Matrix Analysis*. Springer New York, 2012.
- [2] T. S. Ferguson. *A Course in Large Sample Theory*. Taylor & Francis Ltd, 1996.

- [3] G. B. Folland. *Real Analysis*. John Wiley & Sons, 1999.
- [4] J. R. Magnus and H. Neudecker. *Matrix Differential Calculus with Applications in Statistics and Econometrics*. Wiley John & Sons, 2002.
- [5] D. Pollard. *Empirical Processes: Theory and Applications*. Conference Board of the Mathematical Science: NSF-CBMS regional conference series in probability and statistics. Institute of Mathematical Statistics, 1990.
- [6] H. Royden and P. Fitzpatrick. *Real Analysis*. Pearson, 2010.

SCHOOL OF STATISTICS, 313 FORD HALL 224 CHURCH ST SE MINNEAPOLIS, MN 55455, USA  
E-MAIL: [ekvall@umn.edu](mailto:ekvall@umn.edu); [galin@umn.edu](mailto:galin@umn.edu)
